# Supplementary material for: Apples on the Table? Evaluating Text-Guided 3D Scene Synthesis via Fine-Grained Constraint Verification
Source: arXiv:2511.03001 source file (2026-09-01)
Supplement: Supplementary file 1 [file appendix_tools.tex]

\begin{table*}[t]
\centering
\begin{tabular}{cc>{\raggedright\arraybackslash}p{10cm}}
\toprule
\textbf{Tool Types} & \textbf{Tool} & \textbf{Description} \\
\midrule
\multirow{10}{*}{Text} 
 & get room list & Returns a list of room IDs from the given scene. \\
 & get window list & Returns a list of window IDs from the given scene. \\
 & get door list & Returns a list of door IDs from the given scene. \\
 & get wall list & Returns a list of wall IDs from the given scene. \\
 & get object list & Returns a list of object IDs from the given room. \\
 & get room info & Returns detailed information about specific rooms. \\
 & get window info & Returns detailed information about specific windows. \\
 & get door info & Returns detailed information about specific doors. \\
 & get wall info & Returns detailed information about specific walls. \\
 & get object info & Returns detailed information about specific objects. \\
\midrule
\multirow{9}{*}{Visual} 
 & get topdown scene & Returns top-down image of the rendered scene. \\
 & get topdown room & Returns top-down image of the rendered room. \\
 & get material image & Returns images of specified materials. \\
 & get wall scene & Returns images of specified walls. \\
 & get multiview rendered object &  Returns images of the specified objects from multiple angles. \\
 & get topdown object & Returns top-down view images of given objects in the scene. \\
 & get frontview object & Returns front view images of given objects in the scene. \\
 & get spatial relation & Returns top-down scene image with bounding boxes on given objects. \\
\midrule
\multirow{3}{*}{Property} 
 & get object match & Returns mapping of images to its corresponding object in constraint. \\
 & get property description & Returns description of given materials or objects. \\
 & get property verification & Returns constraint-based descriptions of given materials or objects. \\
\bottomrule
\end{tabular}
\caption{Description of tools in our tool set}
\label{tab:List of tools}
\end{table*}
